# Supplementary material for: Treatment-control comparisons in platform trials including non-concurrent controls
Source: arXiv:2407.13546 source file (2024-07-18)
Supplement: Supplementary file 1 [file Suppmaterial.pdf]

# Supplementary Material: “Treatment-control comparisons in platform trials including non-concurrent controls”

Marta Bofill Roig<sup>\*1</sup>, Pavla Krotka<sup>1</sup>, Katharina Hees<sup>2</sup>, Peter Jacko<sup>3,4</sup>, Franz Koenig<sup>1</sup>,  
Dominic Magirr<sup>5</sup>, Tom Parke<sup>3</sup>, and Martin Posch<sup>1</sup>

<sup>1</sup>*Center for Medical Data Science, Medical University of Vienna, Vienna, Austria*

<sup>2</sup>*Section of Data Science and Methods, Paul-Ehrlich-Institut, Langen, Germany*

<sup>3</sup>*Berry Consultants, Abingdon, UK*

<sup>4</sup>*Lancaster University, Lancaster, UK*

<sup>5</sup>*Advanced Methodology and Data Science, Novartis Pharma AG, Basel, Switzerland*

## Contents

|                                                                                            |          |
|--------------------------------------------------------------------------------------------|----------|
| <b>A Additional results from Setting I</b>                                                 | <b>2</b> |
| <b>B Additional results with different prior calibrations for the Time Machine and MAP</b> | <b>5</b> |

---

<sup>\*</sup>marta.bofillroig@meduniwien.ac.at

In this supplementary material, we provide additional results concerning the simulation study. R code to reproduce the results is available at [https://github.com/pavlakrotka/NCC\\_MethodsComp](https://github.com/pavlakrotka/NCC_MethodsComp).

## A Additional results from Setting I

Additional results presented in this supplementary material refer to Setting I.

- Figure 1: Platform trial with three experimental arms, equidistant entry times and equal time trend ( $\lambda_k = 0.15 \forall k$ ).
- Figure 2: Platform trial with three experimental arms, equidistant entry times and different time trends. Two cases of different time trends are included: A) Different time trends in arm 1 only (with  $\lambda_0 = \lambda_2 = \lambda_3 = 0.1$ ) and B) Different time trends in arms 1 and 2 (with  $\lambda_0 = \lambda_3 = 0.1$ ).

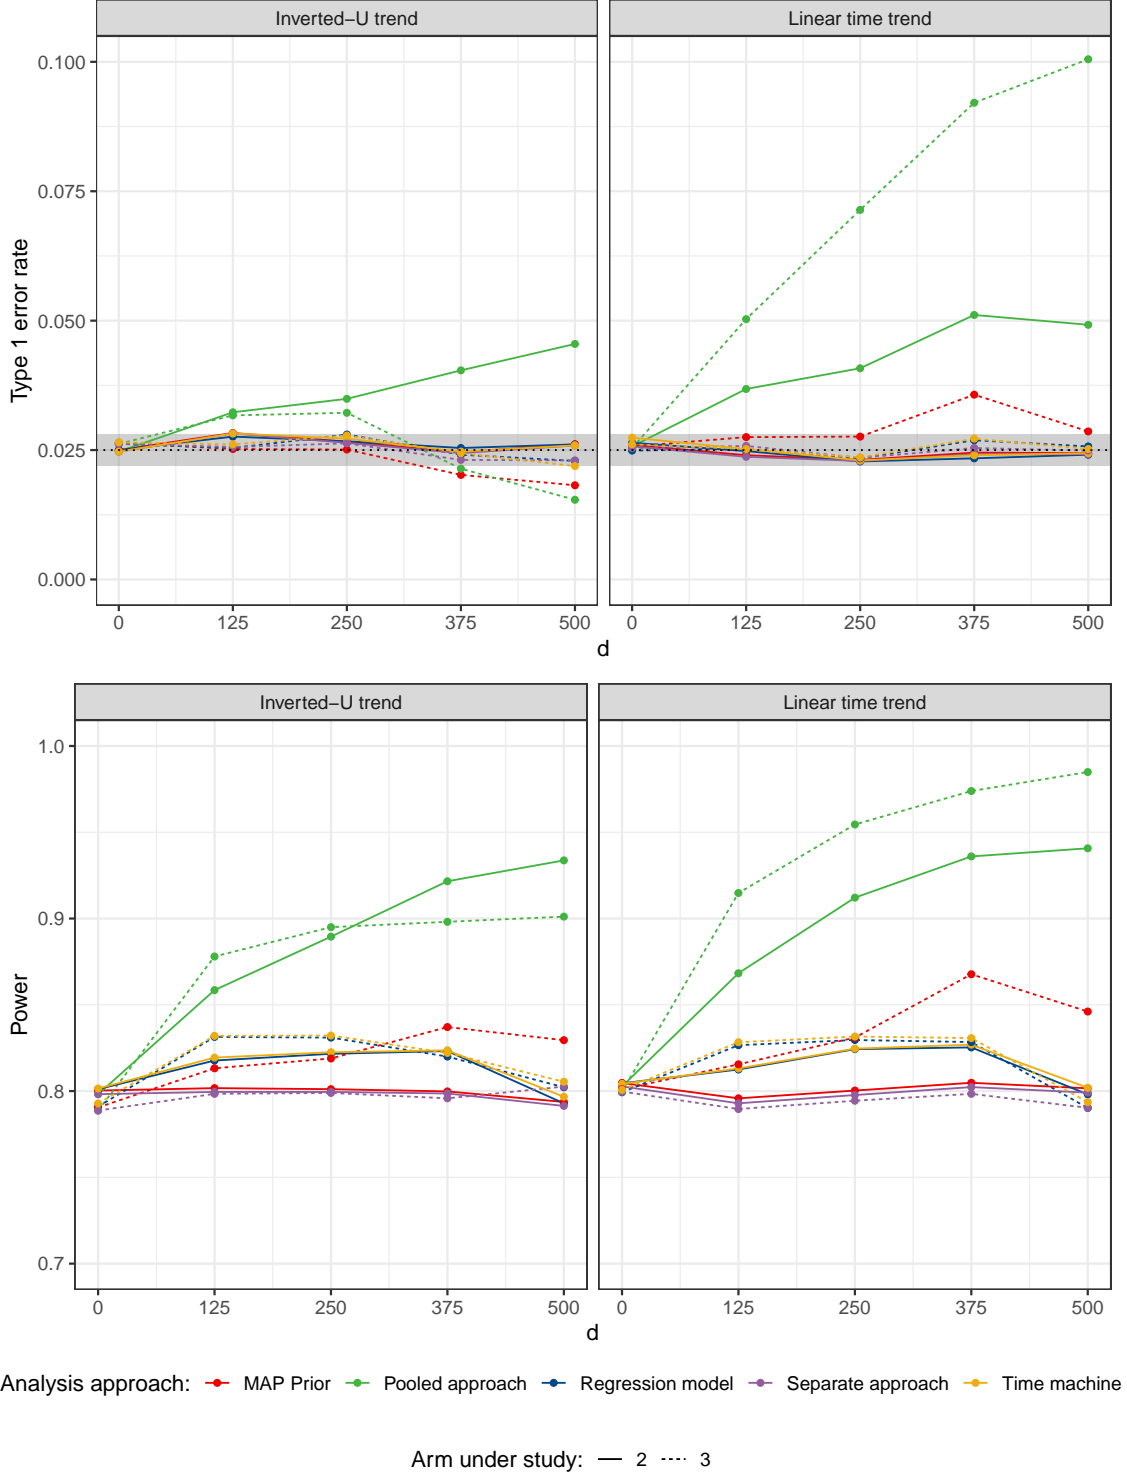

Figure 1: Type 1 error rate (first row) and power (second row) for inverted-U (first column) and linear (second column) time trends ( $\lambda_k = 0.15, \forall k$ ) with respect to the difference in entry time between consecutive arms  $d$  (y-axis) in a setting with three treatment arms (Setting (I), Figure 2 of the main paper) and according to the analysis approach. The straight and dotted lines refer to the results of arms 2 and 3, respectively. Time Machine calibration consists of  $D_{\text{Expected}} = 1$  and  $D_{\text{Maximum}} = 1.5$  according to Table 2 in the main paper. Prior parameters for the MAP prior are set to  $1/\sigma_\beta^2 = 0.001$  and  $1/\sigma_\tau^2 = 0.002$ . The grey area represents the 95% prediction interval of the simulated type 1 error rate with 10,000 replications, provided that the true type 1 error rate is 0.025.

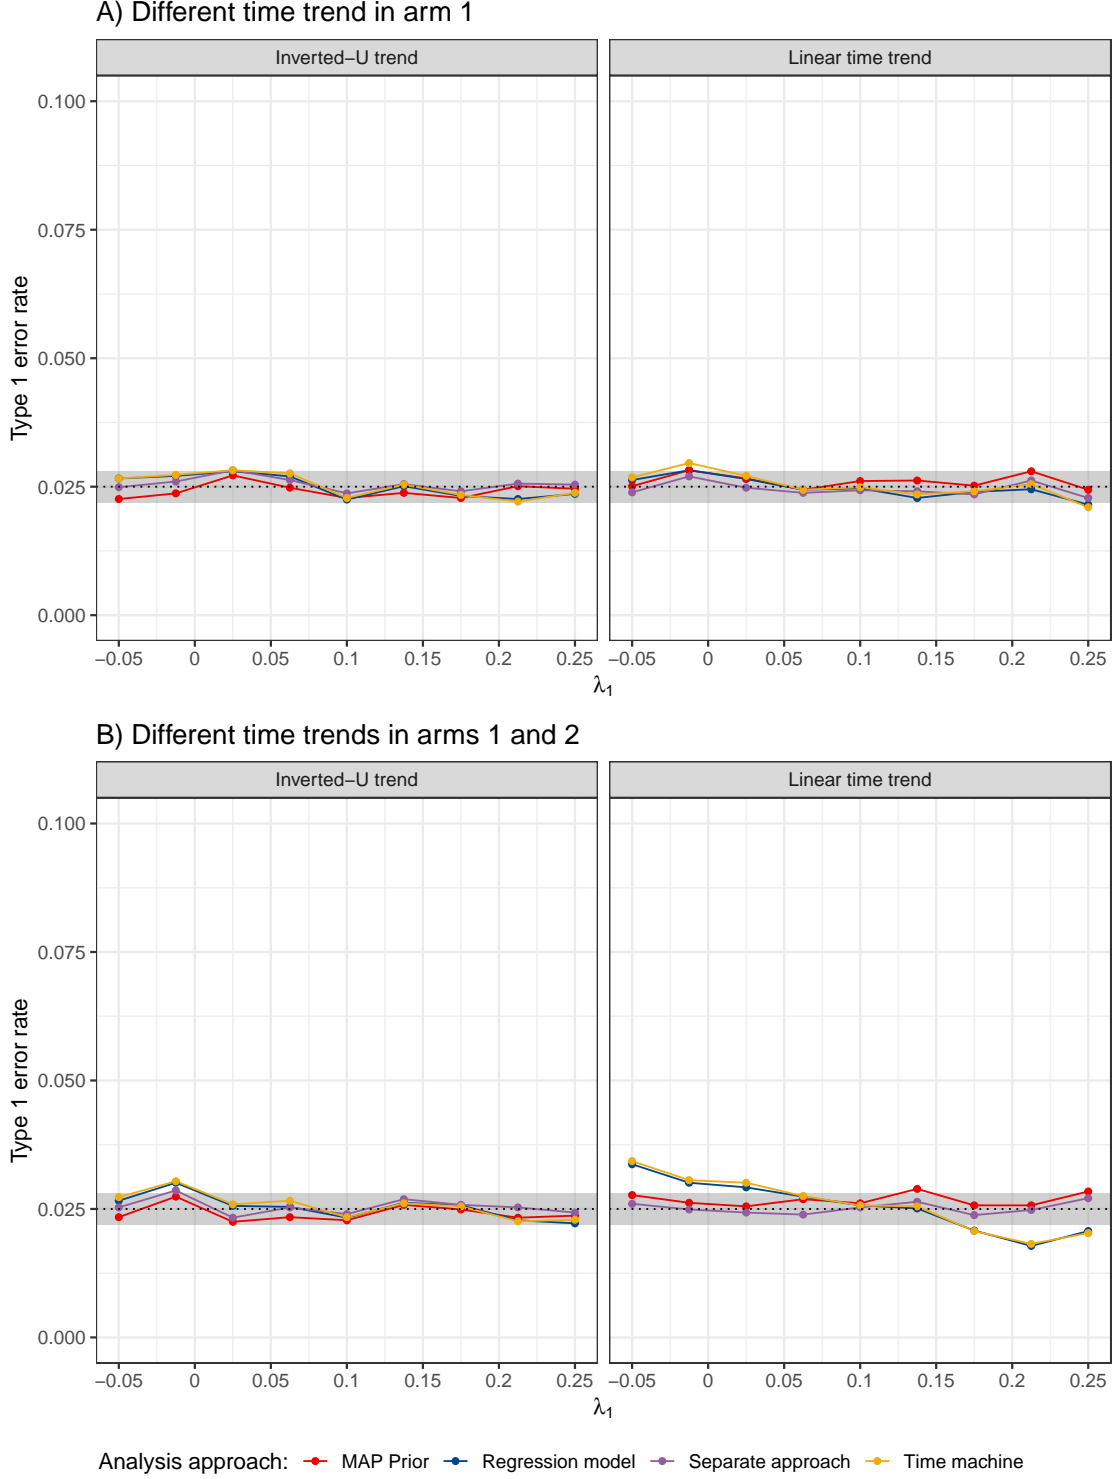

Figure 2: Type 1 error rate of the comparison of arm 3 versus control with respect to the strength of the time trend in arm 1 ( $\lambda_1$ ) in Setting (I) with 3 treatment arms under inverted-U (first column) and linear (second column) time trends according to the analysis approach. In the first row (A), only the time trend for arm 1 differs from the rest ( $\lambda_0 = \lambda_2 = \lambda_3 = 0.1$ ); in the second row (B), time trends for arms 1 and 2 ( $\lambda_1 = \lambda_2$ ) differ from time trends in control and arm 3 ( $\lambda_0 = \lambda_3 = 0.1$ ). Time Machine calibration consists of  $D_{\text{Expected}} = 1$  and  $D_{\text{Maximum}} = 1.5$  according to Table 2 in the main paper. Prior parameters for the MAP prior are set to  $1/\sigma_\beta^2 = 0.001$  and  $1/\sigma_\tau^2 = 0.002$ . The grey area represents the 95% prediction interval of the simulated type 1 error rate with 10,000 replications, provided that the true type 1 error rate is 0.025.

## **B Additional results with different prior calibrations for the Time Machine and MAP**

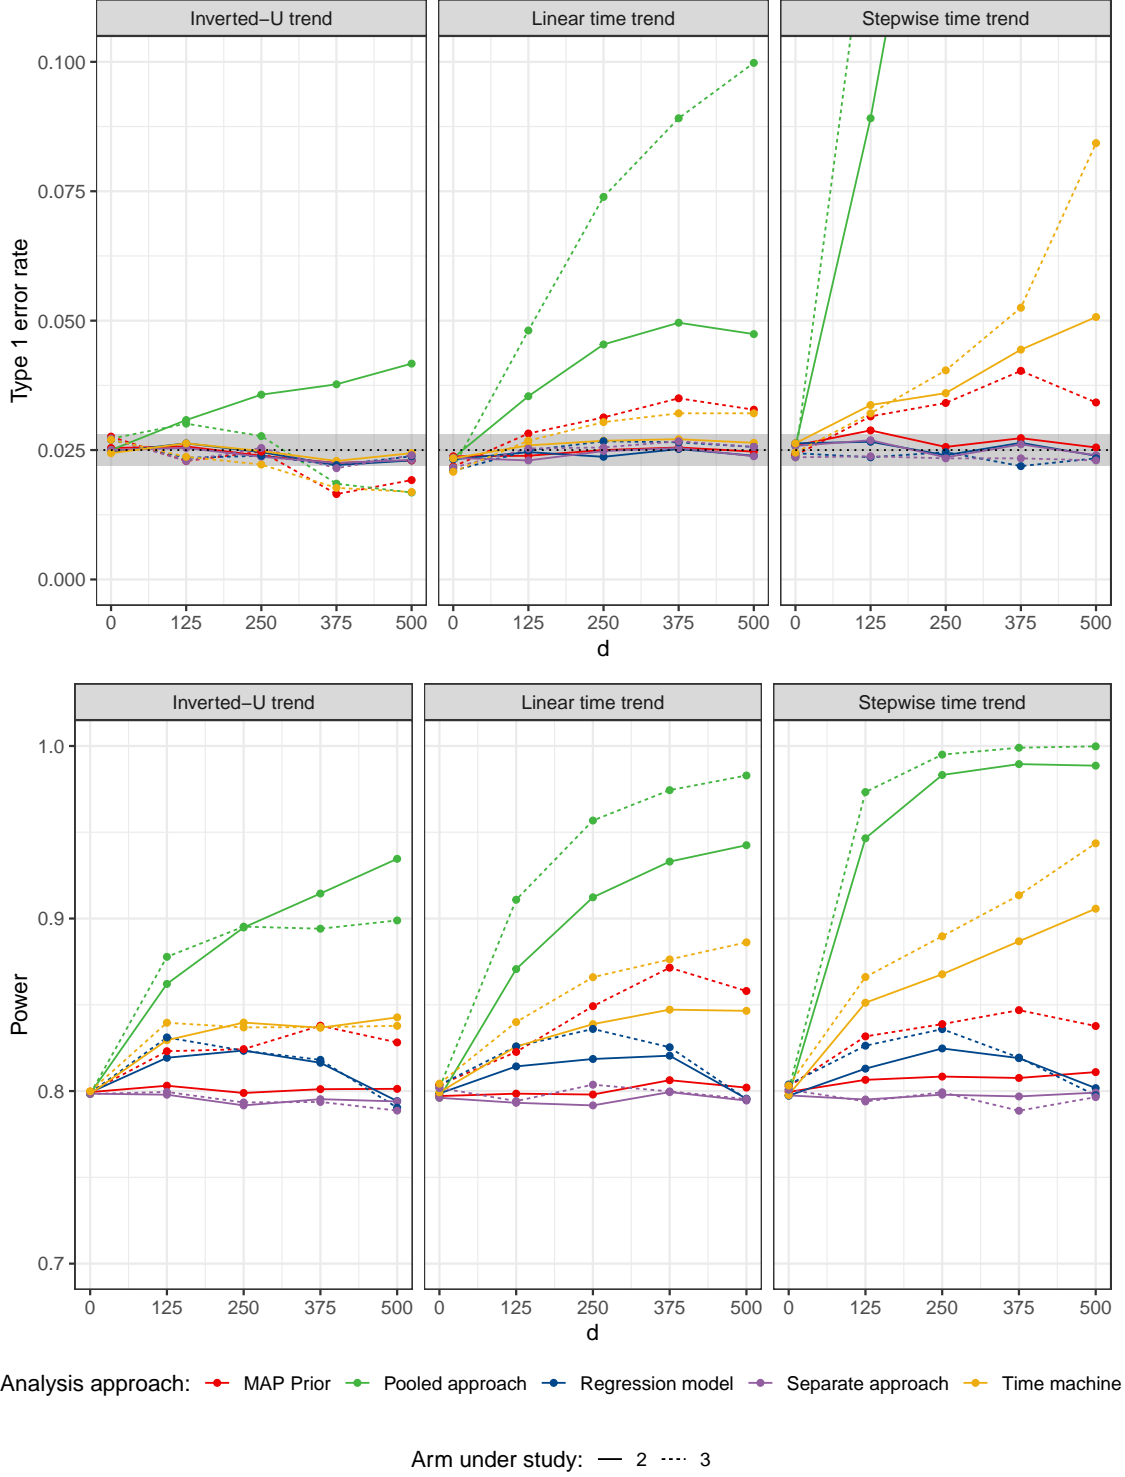

Figure 3: Type 1 error rate (first row) and power (second row) with respect to the difference in entry time between consecutive arms  $d$  (y-axis) in a setting with three treatment arms (Setting (I), Figure 2 of the main paper) and equal time trends ( $\lambda_k = 0.15 \forall k$ ) according to the analysis approach. The straight and dotted lines refer to the results of arms 2 and 3, respectively. Time Machine calibration consists of  $D_{\text{Expected}} = 0.01$  and  $D_{\text{Maximum}} = 0.15$  according to Table 2 in the main paper. Prior parameters for the MAP prior are set to  $1/\sigma_\beta^2 = 1$  and  $1/\sigma_\tau^2 = 0.002$ . The grey area represents the 95% prediction interval of the simulated type 1 error rate with 10,000 replications, provided that the true type 1 error rate is 0.025.

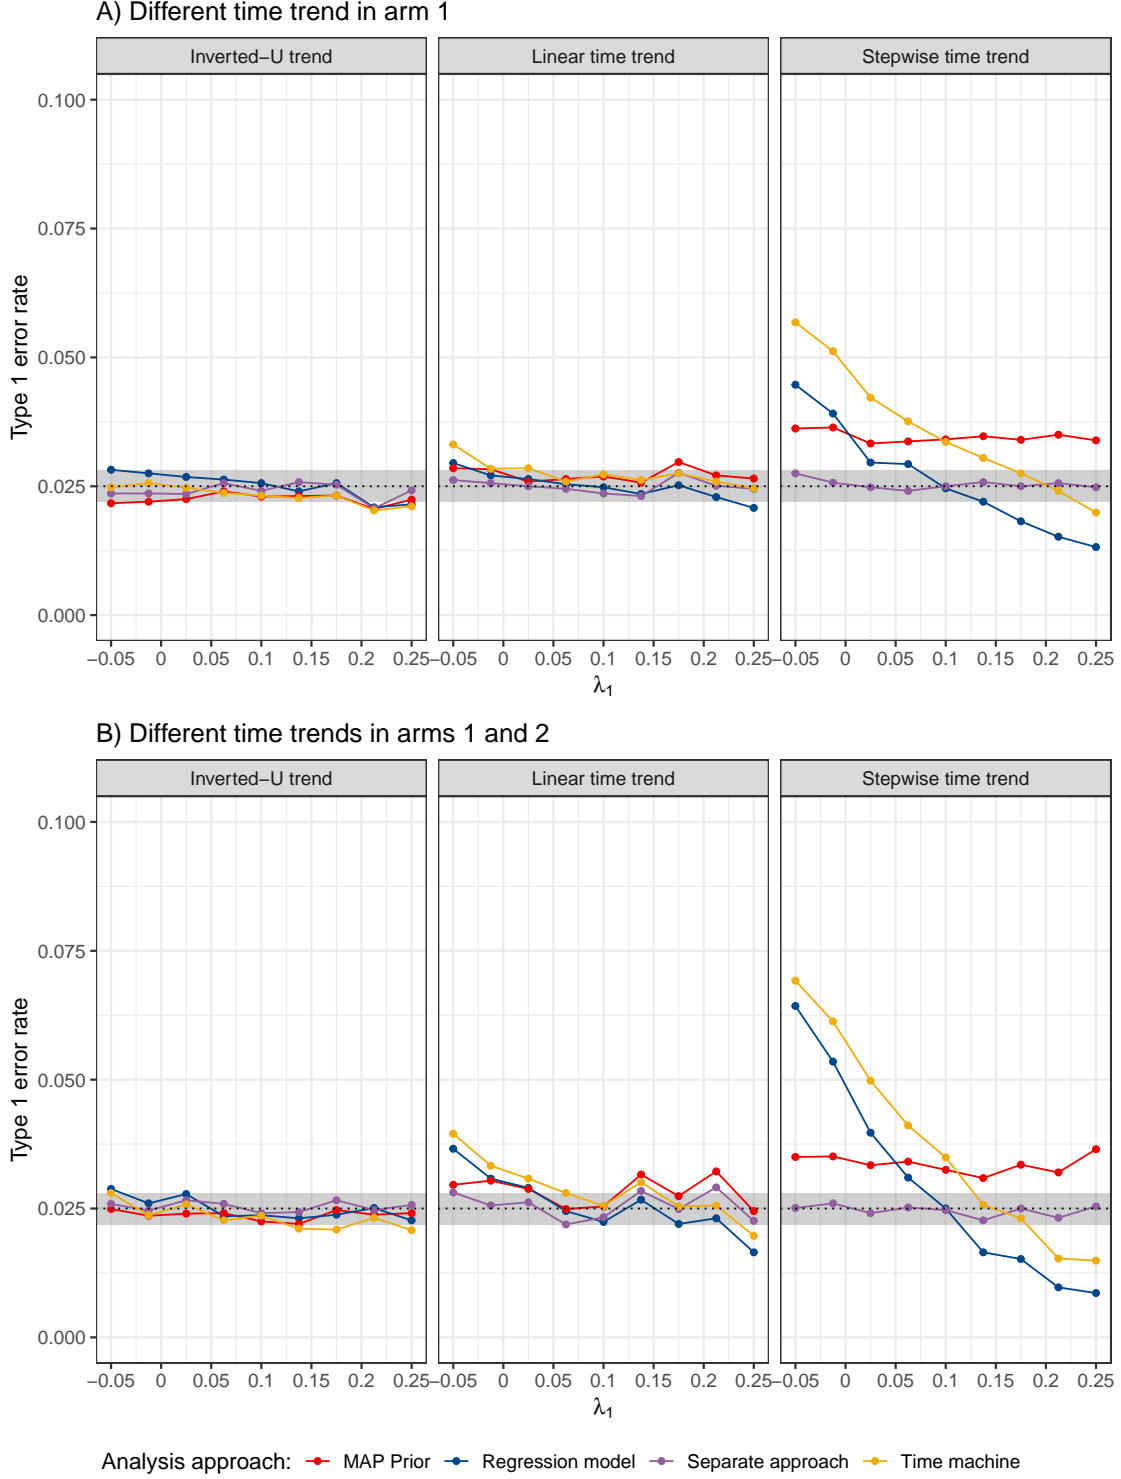

Figure 4: Type 1 error rate of the comparison of arm 3 versus control with respect to the strength of the time trend in arm 1 ( $\lambda_1$ ) in Setting (I) with 3 treatment arms under different time trends according to the analysis approach. In the first row (A), only the time trend for arm 1 differs from the rest ( $\lambda_0 = \lambda_2 = \lambda_3 = 0.1$ ); in the second row (B), time trends for arms 1 and 2 ( $\lambda_1 = \lambda_2$ ) differ from time trends in control and arm 3 ( $\lambda_0 = \lambda_3 = 0.1$ ). Time Machine calibration consists of  $D_{\text{Expected}} = 0.01$  and  $D_{\text{Maximum}} = 0.15$  according to Table 2 in the main paper. Prior parameters for the MAP prior are set to  $1/\sigma_\beta^2 = 1$  and  $1/\sigma_\tau^2 = 0.002$ . The grey area represents the 95% prediction interval of the simulated type 1 error rate with 10,000 replications, provided that the true type 1 error rate is 0.025.

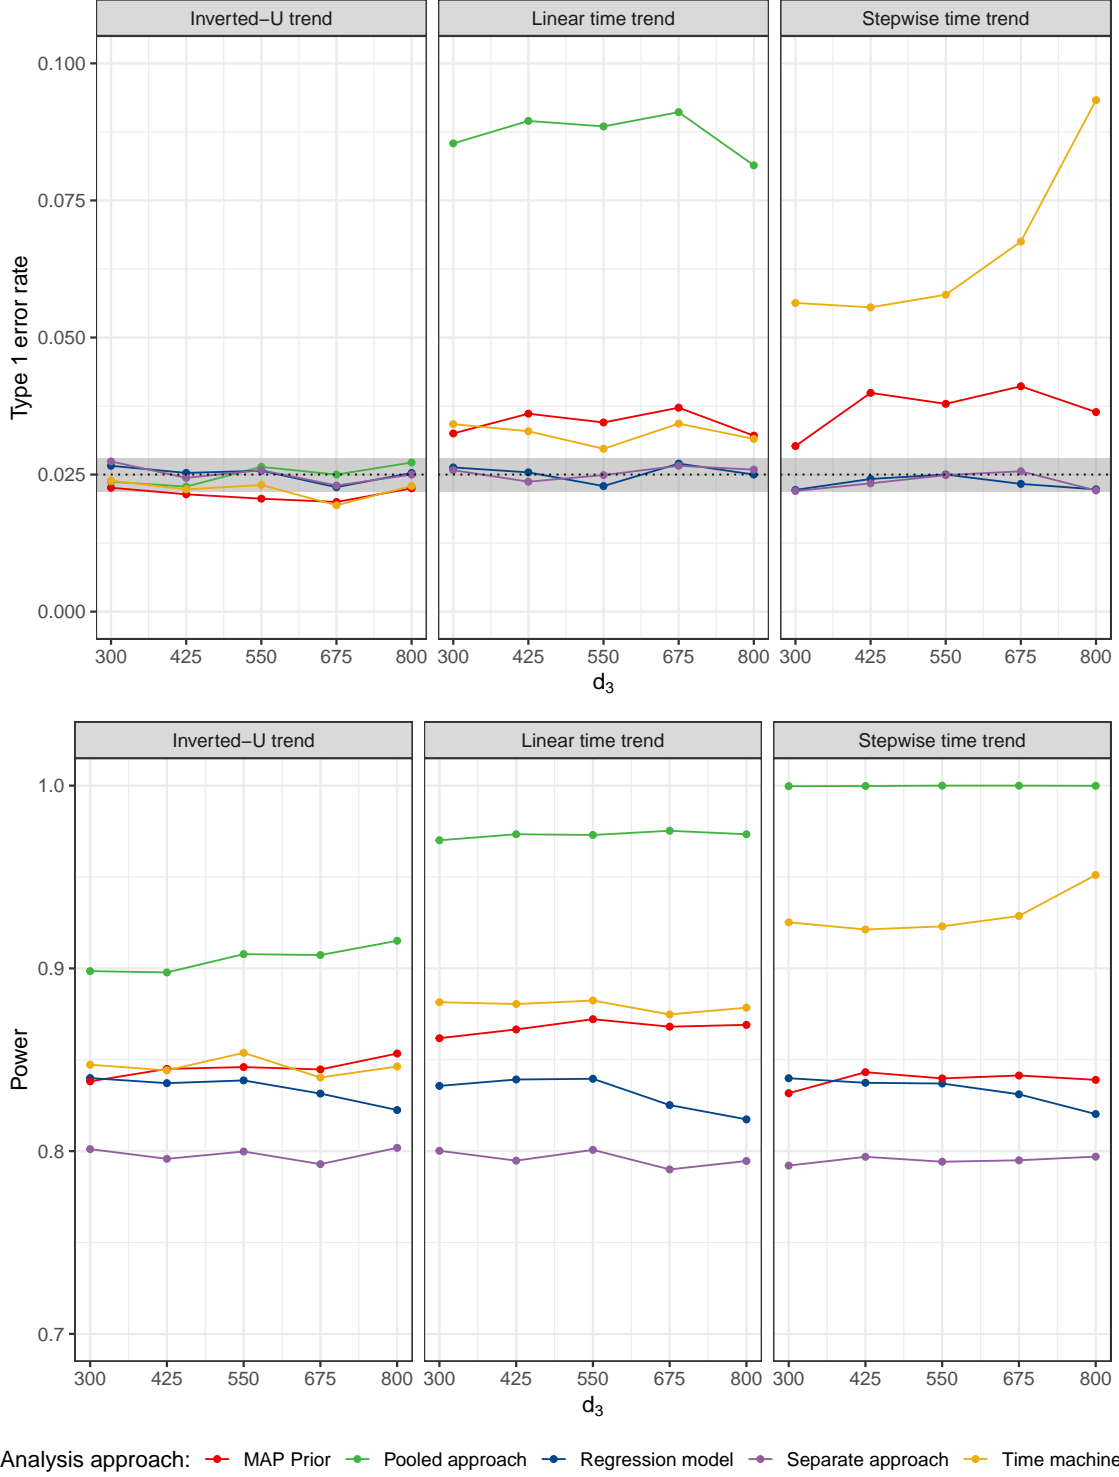

Figure 5: Type 1 error rate (first row) and power (second row) of the comparison of arm 4 against control with respect to the timing of adding the treatment arm 3 ( $d_3$ ) in setting II with four treatment arms and equal time trends ( $\lambda_k = 0.15 \forall k$ ), where arms 2 and 4 enter after  $d_2 = 300$  and  $d_4 = 800$  participants has been allocated to the trial, respectively, according to the analysis approach. Time Machine calibration consists of  $D_{\text{Expected}} = 0.01$  and  $D_{\text{Maximum}} = 0.15$  according to Table 2 in the main paper. Prior parameters for the MAP prior are set to  $1/\sigma_\beta^2 = 1$  and  $1/\sigma_\tau^2 = 0.002$ . The grey area represents the 95% prediction interval of the simulated type 1 error rate with 10,000 replications, provided that the true type 1 error rate is 0.025.



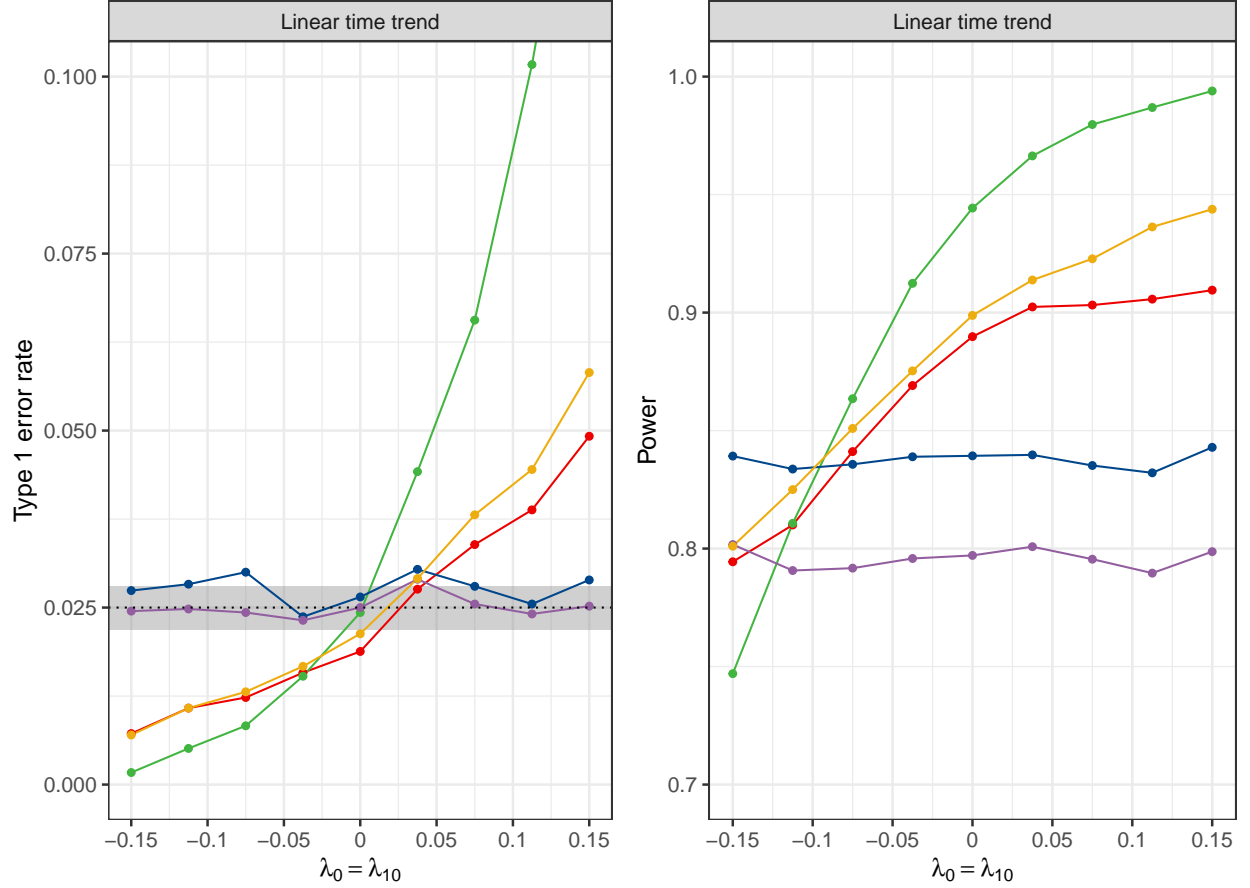

Analysis approach: —•— MAP Prior —•— Pooled approach —•— Regression model —•— Separate approach —•— Time machine

Figure 6: Type 1 error rate (left panel) and power (right panel) of the comparison of arm 10 against control with respect to the strength of the time trend in arm 10 and control ( $\lambda_0 = \lambda_{10}$ ) and according to the analysis approach. These results correspond to setting III with ten treatment arms and different linear time trends, where the time trend for the first 9 arms is sampled from a normal distribution  $N(\lambda_0, 0.5)$ , and the control and arm 10 have equal time trend ( $\lambda_0 = \lambda_{10}$ ). In this setting, a treatment arm  $k$  enters after  $300 \cdot (k - 1)$  participants have been allocated to the trial. Time Machine calibration consists of  $D_{\text{Expected}} = 0.01$  and  $D_{\text{Maximum}} = 0.15$  according to Table 2 in the main paper. Prior parameters for the MAP prior are set to  $1/\sigma_\beta^2 = 1$  and  $1/\sigma_\tau^2 = 0.002$ . The grey area represents the 95% prediction interval of the simulated type 1 error rate with 10,000 replications, provided that the true type 1 error rate is 0.025.
